# Supplementary material for: Spherical wedge billiard: from chaos to fractals and Talbot carpets
Source: arXiv:2209.03096 ancillary file (2022-09-07)
Supplement: Supplementary file 1 [file analysis_of_ellipses.pdf]

# Supplemental Material for: “The spherical wedge billiard: a non-Euclidean system exhibiting complex behavior”

Tomáš Tyc and Darek Cidliński

## ELLIPSES IN THE PHASE SPACE DIAGRAM FOR THE BILLIARD PARAMETER $\Phi$ CLOSE TO $\pi$

### Iterating the Poincaré map multiple steps

In the following we investigate the Poincaré map  $M$  for the billiard parameter  $\Phi$  close to  $\pi$ . We will show that for an integer  $n > 1$ , there is a fixed point of the mapping  $M^{2n}$  near the point  $(\xi, \omega) = (0, \pi/(2n))$ . We will find the position of this point and investigate the phase space diagram in the vicinity of this point; we will show that the phase space diagram in the plane  $(\xi, \omega)$  contains stacks of ellipses.

To shorten the notation, in the following equations we drop the symbol “mod  $2\pi$ ” used in the main paper; this way, if any expression results in a value from outside the interval  $(-\pi, \pi]$ , it is automatically increased or decreased by  $2\pi$  to belong to this interval.

We set  $\Phi = \pi - \varepsilon$  with  $\varepsilon \ll 1$  and expand Eqs. (1–2) from the main paper in  $\varepsilon$ , keeping terms up to the first order in  $\varepsilon$ . We denote  $s_k \equiv \text{sign}[\sin(\vartheta_k - 2\omega_k)] = \text{sign}[\sin(\xi_k - \omega_k)]$  to shorten notation, and employ Taylor expansion. This yields

$$\vartheta_{k+1} = \frac{\pi s_k}{2} - \arctan \left\{ \cot(\vartheta_k - 2\omega_k) + \frac{\varepsilon s_k \tan \omega_k}{\sin(\vartheta_k - 2\omega_k)} \right\} = \vartheta_k - 2\omega_k - \varepsilon s_k \sin(\vartheta_k - 2\omega_k) \tan \omega_k, \quad (\text{S1})$$

$$\omega_{k+1} = -\arcsin\{-\sin \omega_k + \varepsilon s_k \cos \omega_k \cos(\vartheta_k - 2\omega_k)\} = \omega_k - \varepsilon s_k \cos(\vartheta_k - 2\omega_k). \quad (\text{S2})$$

With the help of Eqs. (3) from the main paper, we rewrite these equations in terms of the variables  $(\xi, \omega)$  instead of  $(\vartheta, \omega)$ :

$$\xi_{k+1} = \xi_k - 2\omega_k + \varepsilon s_k \frac{\cos \xi_k}{\cos \omega_k} \quad (\text{S3})$$

$$\omega_{k+1} = \omega_k - \varepsilon s_k \cos(\xi_k - \omega_k) \quad (\text{S4})$$

We now wish to iterate Eqs. (S3) and (S4), starting from the point  $(\xi_0, \omega_0) = (0, \pi/(2n))$ , by  $n$  steps forward. To do that, we use the fact that for small  $\varepsilon$ , the resulting sequence of points  $\{(\xi_k, \omega_k), k = 1, \dots, n\}$  will be close to the sequence  $\{(\tilde{\xi}_k, \tilde{\omega}_k), k = 1, \dots, n\}$  of points that would correspond to a similar iteration with the same starting point  $(\xi_0, \omega_0)$ , but with  $\varepsilon = 0$ . This latter sequence can be obtained easily by using  $\varepsilon = 0$  in Eqs. (S3) and (S4) and iterating, which gives  $\tilde{\xi}_k = \xi_0 - 2k\omega_0$  and  $\tilde{\omega}_k = \omega_0$ . Now, when calculating the sequence  $\{(\xi_k, \omega_k)\}$ , we use Eqs. (S3) and (S4) where in the terms containing  $\varepsilon$  we replace  $\xi_k$  and  $\omega_k$  by their approximate values  $\tilde{\xi}_k$  and  $\tilde{\omega}_k$ ; doing that, we introduce an error of order  $\varepsilon^2$ , which is no problem because we are calculating up to the first order in  $\varepsilon$ . This way, we obtain

$$\xi_{k+1} = \xi_k - 2\omega_k + \varepsilon s_k \frac{\cos(\xi_0 - 2k\omega_0)}{\cos \omega_0}, \quad (\text{S5})$$

$$\omega_{k+1} = \omega_k - \varepsilon s_k \cos[\xi_0 - (2k+1)\omega_0]. \quad (\text{S6})$$

We now go  $n$  steps forward. By repeatedly using the recurrence (S5–S6), we obtain

$$\begin{aligned} \xi_n &= \xi_0 - 2n\omega_0 + \frac{\varepsilon}{\cos \omega_0} \sum_{k=0}^{n-1} s_k \cos(\xi_0 - 2k\omega_0) + 2\varepsilon \sum_{k=0}^{n-1} (n-k-1) s_k \cos[\xi_0 - (2k+1)\omega_0], \\ \omega_n &= \omega_0 - \varepsilon \sum_{k=0}^{n-1} s_k \cos[\xi_0 - (2k+1)\omega_0]. \end{aligned} \quad (\text{S7})$$

As we have mentioned, we want to start our iteration near the point  $(\xi, \omega) = (0, \pi/(2n))$  (but not necessarily exactly at that point). This way, we have  $\xi_0 \approx 0$  and  $\omega_0 \approx \frac{\pi}{2n}$ . Then since  $\xi_k - \omega_k \approx \xi_0 - (2k+1)\omega_0 \approx -\frac{(2k+1)\pi}{2n}$ , we see that

all the signs  $s_0, s_1, \dots, s_{n-1}$  are equal to  $-1$ . This makes it possible to rewrite (S7) to

$$\begin{aligned}\xi_n &= \xi_0 - 2n\omega_0 - \frac{\varepsilon}{\cos \omega_0} \sum_{k=0}^{n-1} \cos(\xi_0 - 2k\omega_0) - 2\varepsilon(n-1) \sum_{k=0}^{n-1} \cos[\xi_0 - (2k+1)\omega_0] + 2\varepsilon \sum_{k=0}^{n-1} k \cos[\xi_0 - (2k+1)\omega_0], \\ \omega_n &= \omega_0 + \varepsilon \sum_{k=0}^{n-1} \cos[\xi_0 - (2k+1)\omega_0].\end{aligned}\tag{S8}$$

Evaluating the sums is a technical task. After a lot of algebra, we find

$$\begin{aligned}\xi_n &= \xi_0 - 2n\omega_0 + \frac{\varepsilon}{\sin \omega_0} \left[ \frac{\sin(n\omega_0) \sin(\xi_0 - n\omega_0)}{\sin \omega_0 \cos \omega_0} - n \sin \xi_0 \right], \\ \omega_n &= \omega_0 + \varepsilon \frac{\cos(\xi_0 - n\omega_0) \sin(n\omega_0)}{\sin \omega_0},\end{aligned}\tag{S9}$$

### Finding the fixed point of the map $M^{2n}$

As we have mentioned, we are looking for a fixed point of the mapping  $M^{2n}$  near the point  $(\xi, \omega) = (0, \pi/(2n))$ . Instead of iterating the full  $2n$  steps forward, we instead compare the result of iterating just  $n$  steps forward with the result of iterating  $n$  steps backward. By requiring that the result be the same, we obtain the position of the fixed point of the mapping  $M^{2n}$ . Compared to iterating  $2n$  steps forward, this more symmetric approach leads to equations of a simpler form for the fixed point than the iteration by  $2n$  steps would lead to. Therefore we prefer this approach.

It is not difficult to find the relations for the backward iteration analogous to Eqs. (S3) and (S4) based on symmetry consideration of the spherical wedge billiard and the resulting symmetries of the Poincaré map  $M$  in the plane  $(\xi, \omega)$ ; we omit these considerations here and just state the result:

$$\begin{aligned}\xi_{-n} &= \xi_0 + 2n\omega_0 + \frac{\varepsilon}{\sin \omega_0} \left[ \frac{\sin(n\omega_0) \sin(\xi_0 + n\omega_0)}{\sin \omega_0 \cos \omega_0} - n \sin \xi_0 \right], \\ \omega_{-n} &= \omega_0 + \varepsilon \frac{\cos(\xi_0 + n\omega_0) \sin(n\omega_0)}{\sin \omega_0}.\end{aligned}\tag{S10}$$

We can now express the differences of the result of  $n$  iterations forward and  $n$  iterations backward as

$$\xi_n - \xi_{-n} = -4n\omega_0 - 4\varepsilon \frac{\sin^2 n\omega_0 \cos \xi_0}{\sin \omega_0 \sin 2\omega_0},\tag{S11}$$

$$\omega_n - \omega_{-n} = 2\varepsilon \frac{\sin^2 n\omega_0}{\sin \omega_0} \sin \xi_0.\tag{S12}$$

The requirement that the point  $(\xi_0, \omega_0)$  is a fixed point of the mapping  $M^{2n}$  is equivalent to requiring  $\xi_n = \xi_{-n}$  and  $\omega_n = \omega_{-n}$ , so the right-hand sides of Eqs. (S11) and (S12) must vanish. The second condition is clearly satisfied by  $\xi_0 = 0$ . Writing  $\omega_0 = \pi/(2n) + b$ , after a bit of algebra the first condition yields the following equation for  $b$

$$b = -\frac{\varepsilon \cos^2 nb}{n \sin(\frac{\pi}{2n} + b) \sin(\frac{\pi}{n} + 2b)}.\tag{S13}$$

Taking into account that  $b$  is of order of  $\varepsilon$  as Eq. (S13) shows, we can get neglect all  $b$  on the right-hand side of Eq. (S13), which gives  $b$  up to the first order in  $\varepsilon$  as  $b = -\varepsilon/(n \sin \frac{\pi}{n} \sin \frac{\pi}{2n})$ . So finally we can write the coordinates of the fixed point of the mapping  $M^{2n}$  that we denote by  $F = (\xi_F, \omega_F)$  as follows:

$$\xi_F = 0, \quad \omega_F = \frac{\pi}{2n} - \frac{\varepsilon}{n \sin \frac{\pi}{n} \sin \frac{\pi}{2n}}\tag{S14}$$

This result is in an excellent agreement with numerical calculations with an error of the second order in  $\varepsilon$ , as expected. We also note that the position of one fixed point of  $M^{2n}$  given by Eq. (S14) can be used to find the positions of all the  $2n - 1$  other fixed points with the help of Eqs. (S9) and (S10), i.e., we can recover the whole  $2n$ -periodic orbit up to the first order in  $\varepsilon$ . Another important fixed point of this mapping is the one that is a result of applying the mapping  $M^n$  to the fixed point  $F$  we have found, i.e., the point  $F' = (\xi'_F, \omega'_F) = M^n F$ . It is not hard to see that this point has the same  $\omega$  coordinate as the fixed point  $F$  while its  $\xi$  coordinate differs by  $\pi$ ; this way, we can write  $F' = (\pi, \frac{\pi}{2n} - \varepsilon/[n \sin \frac{\pi}{n} \sin \frac{\pi}{2n}])$ .

### Getting equations for the ellipses

Having found the fixed points of the mapping  $M^{2n}$ , it remains to find the relation between the difference  $(\xi_{-n}, \omega_{-n}) - F'$  of the original point and the fixed point and the difference  $(\xi_n, \omega_n) - F'$  of the resulting point and the fixed point; this relation is described by the Jacobi matrix

$$J_{2n} = \begin{pmatrix} \frac{\partial \xi_n}{\partial \xi_{-n}} & \frac{\partial \xi_n}{\partial \omega_{-n}} \\ \frac{\partial \omega_n}{\partial \xi_{-n}} & \frac{\partial \omega_n}{\partial \omega_{-n}} \end{pmatrix} \quad (\text{S15})$$

expressed at the fixed point. With the help of Eqs. (S9) and (S10) we can calculate  $J_{2n}$  up to the first order in  $\varepsilon$ :

$$J_{2n} = \begin{pmatrix} 1 - \frac{4n\varepsilon}{\sin[\pi/(2n)]} & -4n + \varepsilon f(n) \\ \frac{2\varepsilon}{\sin[\pi/(2n)]} & 1 - \frac{4n\varepsilon}{\sin[\pi/(2n)]} \end{pmatrix}, \quad (\text{S16})$$

where  $f(n)$  is a function of  $n$  that can be evaluated explicitly but whose form is not important for our considerations. We now perform a specific similarity transformation of this matrix:

$$\tilde{J}_{2n} \equiv \begin{pmatrix} 1 & 0 \\ 0 & 1/R_n \end{pmatrix} J_{2n} \begin{pmatrix} 1 & 0 \\ 0 & R_n \end{pmatrix}, \quad (\text{S17})$$

where  $R_n = \sqrt{\varepsilon/\{2n \sin[\pi/(2n)]\}}$ . The matrix  $\text{diag}(1, 1/R_n)$  in Eq. (S17) effectively scales the coordinate  $\omega$  by the factor  $1/R_n$ , so the transformed matrix  $\tilde{J}_{2n}$  can be regarded as the Jacobi matrix of the mapping  $M^{2n}$  in the rescaled coordinates  $(\xi, \omega/R_n)$ . A direct calculation using Eqs. (S16) and (S17) shows that, up to the first order in  $\varepsilon$ , the matrix  $\tilde{J}_{2n}$  is just the rotation matrix:

$$\tilde{J}_{2n} = \begin{pmatrix} \cos \alpha_n & -\sin \alpha_n \\ \sin \alpha_n & \cos \alpha_n \end{pmatrix}, \quad (\text{S18})$$

where  $\alpha_n = \sqrt{8n\varepsilon/\sin[\pi/(2n)]}$ . This way, in the rescaled coordinates  $(\xi, \omega/R_n)$  the mapping  $M^{2n}$  simply rotates the neighborhood of the fixed point  $F'$  by the angle  $\alpha_n$  around  $F'$ . And similarly, in the same coordinates the mapping  $M^{2n}$  rotates the neighborhood of the fixed point  $F$  by the angle  $\alpha_n$  around  $F$ . Using this latter fact, we can express the sequence of points  $(\xi_{2nk}, \omega_{2nk})$  corresponding to iterations by the mapping  $M^{2n}$  in the original plane  $(\xi, \omega)$  as

$$\begin{aligned} \xi_{2nk} &= \xi_F + A \cos(k\alpha_n + \phi_0) = A \cos(k\alpha_n + \phi_0), \\ \omega_{2nk} &= \omega_F + AR_n \sin(k\alpha_n + \phi_0) = \frac{\pi}{2n} - \frac{\varepsilon}{n \sin \frac{\pi}{n} \sin \frac{\pi}{2n}} + AR_n \sin(k\alpha_n + \phi_0), \end{aligned} \quad (\text{S19})$$

where  $A$  is an amplitude [radius of a circle in the plane  $(\xi, \omega/R_n)$ ] and  $\phi_0$  denotes the initial phase. This way, the orbit of the mapping  $M^{2n}$  in the plane  $(\xi, \omega/R_n)$  in the neighborhood of the fixed point  $F$  consists of points lying on a circle of radius  $A$  centered at the fixed point  $F$ , with a constant angle  $\alpha_n$  separating two subsequent points. In the original plane  $(\xi, \omega)$  the corresponding points lie along ellipses with axis ratio  $R_n$ . This is the reason that for small  $\varepsilon$ , i.e., for  $\Phi$  just slightly less than  $\pi$ , the phase space diagram consists of plethora of ellipses. Here we have focused on just a subset of all these ellipses; similar considerations as the ones made here would lead to description of the other ellipses too. In particular, one would find that there are infinitely many other stacks of ellipses centered near the points  $(\xi, \omega) = (0, m\pi/(2n))$ , where  $n$  and  $m < n$  are relatively prime. The size and axes ratio of a given stack depends only on  $n$ , but not  $m$ ; the size of the stacks in the  $\xi$  direction is approximately  $\pi/n$ , so it decreases with an increasing denominator of the fraction  $m/n$ . This way, the arrangement of the stacks of ellipses along the  $\omega$  axis in the SWB reflects the structure of rational numbers within the set of real numbers. A similar structure can be found in the fractional Talbot effect where at the distance given by the ratio  $m/n$  of the Talbot length behind the diffraction grating, there is a superposition of  $n$  mutually shifted copies of the original grating.

Fig. S1 shows the phase space diagrams for several values of  $\varepsilon$ . The ratio of the scales on the axes  $\xi$  and  $\omega$  is chosen to be  $R_{n \rightarrow \infty} = \sqrt{\varepsilon/\pi}$  so that the ellipses corresponding to large  $n$  are almost circles.

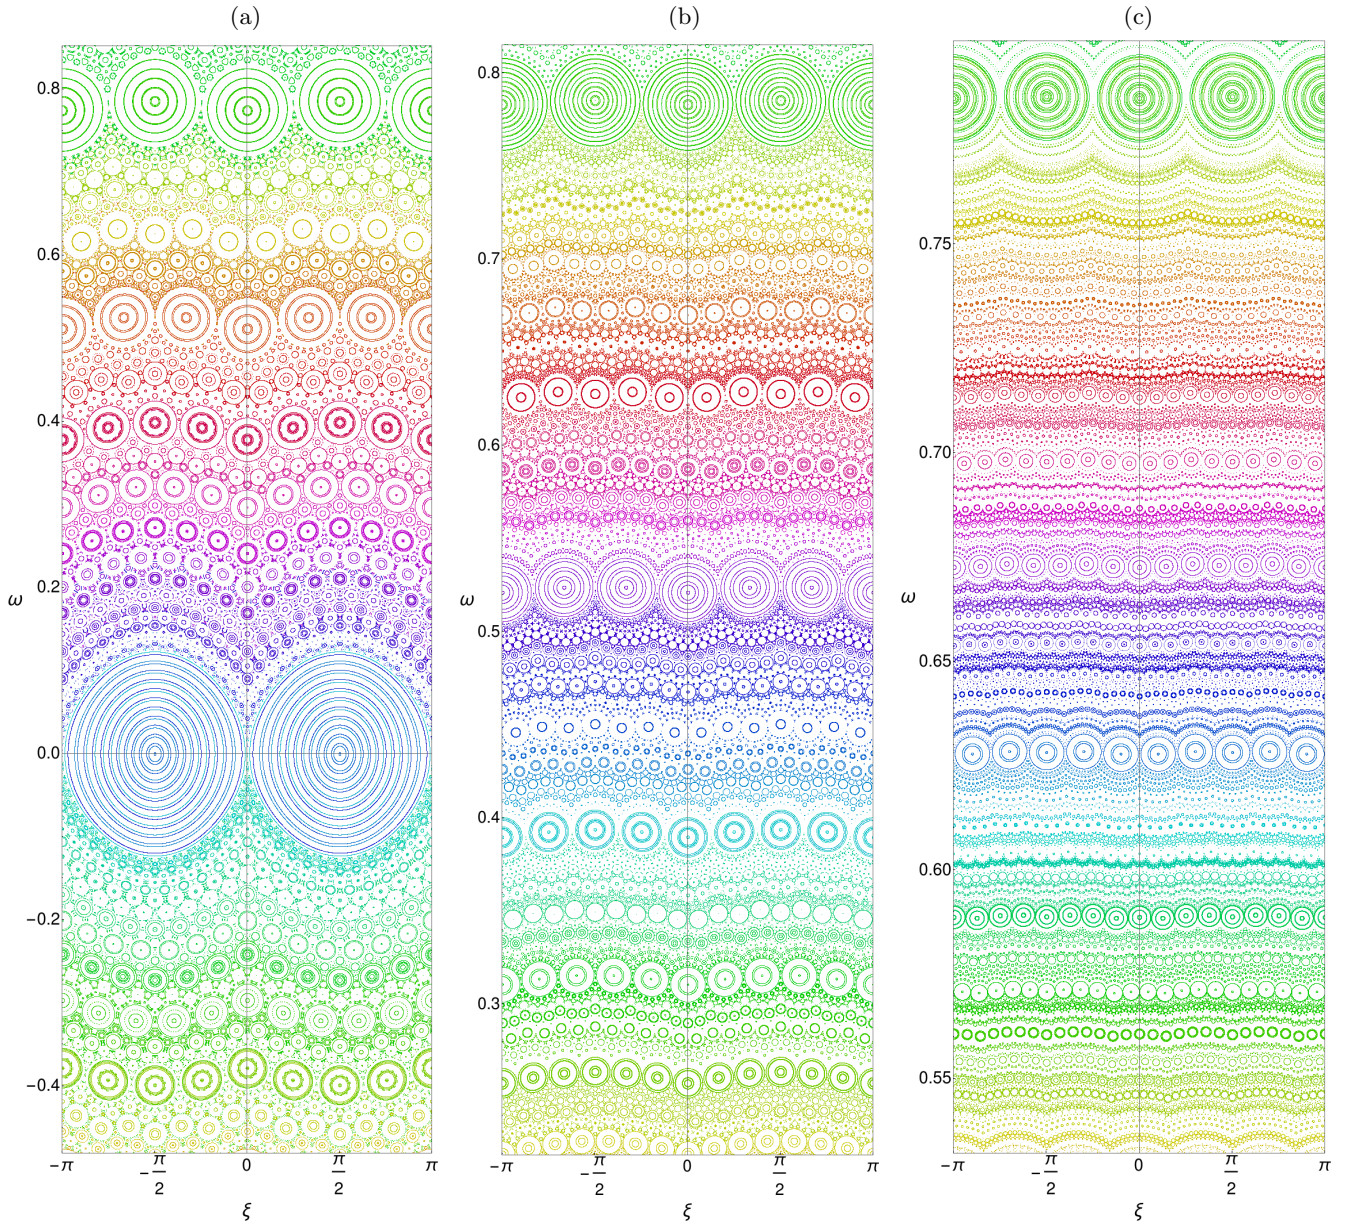

FIG. S1. The phase space diagrams for  $\Phi$  close to  $\pi$ , for several values of  $\varepsilon = \pi - \Phi$ : (a)  $\varepsilon = 0.005\pi$ , (b)  $\varepsilon = 0.001\pi$ , (c)  $\varepsilon = 0.0002\pi$ . The ratio of the scales on the axes  $\xi$  and  $\omega$  is chosen such that most of the ellipses look like circles. The uppermost set of four ellipses located near  $\omega = \pi/4$  corresponds to  $n = 2$  as discussed above.
